# Supplementary material for: TalentRL: Strategy-Guided Reinforcement Learning for Hierarchical Skill Routing
Source: arXiv:2610.41143 source file (2026-10-30)
Supplement: Supplementary file 2 [file additional_experiment_tables.tex]

\begin{table}[ht]
\caption{Matched-seed strict Search7 macro exact match (\%) for routing-credit
variants. $\Delta$ is mixed minus the no-prior-only ablation. The final row
reports the mean and sample standard deviation over the three completed
pairs.}
\label{tab:matched-credit}
\centering
\small
\begin{tabular}{lrrr}
\toprule
Seed & Mixed credit & No-prior-only credit & $\Delta$ \\
\midrule
0 & 41.95 & 41.25 & +0.69 \\
2 & 42.70 & 40.83 & +1.87 \\
3 & 40.73 & 40.32 & +0.41 \\
\midrule
Mean $\pm$ std. & $41.79\pm0.99$ & $40.80\pm0.47$ & +0.99 \\
\bottomrule
\end{tabular}
\end{table}
